# Supplementary material for: PoseAug: A Differentiable Pose Augmentation Framework for 3D Human Pose Estimation
Source: arXiv:2105.02465 source file (2021-05-06)
Supplement: Supplementary file 1 [file appendix.tex]

\newpage
\appendix

\section{Implementation details} \label{sec:Implementation-details}
The pose estimator $\mathcal{P}$ mainly consists 4 residual blocks (RB) proposed in~\cite{pavllo2019videopose3d}. Each RB consists of two 1x1 1D Conv.,
Batch Normalization (BN)~\cite{ioffe2015batch}, ReLU and dropout~\cite{srivastava2014dropout} with residual connection \cite{He_2016_CVPR}. The feature dimension and dropout rate are set as 1024 and 0.25, respectively.
The pose augmentor consists of four linear layers with Batch Normalization (BN) and leaky ReLU~\cite{he2015delving} to first transforms the input 3D pose $\boldsymbol{X}$ to hidden features (256-dim), and then regresses the augmentation parameters $\boldsymbol{\gamma_{ba}}$, $\boldsymbol{\gamma_{bl}}$, $\boldsymbol{R}$ and $\boldsymbol{T}$ from the hidden features respectively.
Both the 3D and 2D pose discriminators consist of 4 linear layers with leaky ReLU and residual connection. The feature dimensions are set as 256 and 100 for 3D and 2D discriminator, respectively.
We train our model for 50 epochs on Human3.6M, with batch size of 1024. We adopt Adam optimizer~\cite{kingma2014adam} with linear decay and an initial learning rate of 0.001 for all networks. The hard ratio $\beta$ linearly increases from 2 to 20 during the training process. The threshold for regularizing the augmentation parameters $\boldsymbol{\gamma_{ba}}$ and $\boldsymbol{\gamma_{bl}}$ are set as $0.1$.

\begin{algorithm}[!h]
\caption{Training Strategy in PoseAug}
\KwIn{training  $\{{\boldsymbol{x}}_i, {\boldsymbol{X}}_i\}_{i=1}^M$, and
the number of training epochs $S$.}
\KwOut{pose estimator $\mathcal{P}$, augmentor $\mathcal{A}$ and discriminator $\mathcal{D}$.}
\For{$s=1,\cdots,S$}
{
    \For{$i=1,\cdots,M$}
    {
        \vspace*{3mm}
        \emph{// Update augmentor $\mathcal{A}$ and discriminator $\mathcal{D}$}\\
        Generate augmented sample $\{{\boldsymbol{x}'}_i, {\boldsymbol{X}'}_i\}$ from $\{{\boldsymbol{x}}_i, {\boldsymbol{X}}_i\}$\\
        Calculate the augmentor and discrimination losses using Eqn.~\eqref{eq:poseloss} to  \eqref{eq:d-loss} \\
        Update the learnable parameters in $\mathcal{A}$ and $\mathcal{D}$\\
        \vspace*{3mm}
    }
    
    \emph{// Update estimator $\mathcal{P}$}\\
    Calculate the estimator loss using Eqn.~\eqref{eq:poseloss} by feeding $\{{\boldsymbol{x}}_i, {\boldsymbol{X}}_i\}_{i=1}^M$ and $\{{\boldsymbol{x}'}_i, {\boldsymbol{X}'}_i\}_{i=1}^M$ to $\mathcal{P}$\\
    Update the learnable parameters in $\mathcal{P}$\\
}
\label{alg:algorithm}
\end{algorithm}
